# Supplementary material for: Detecting and monitoring long-term landslides in urbanized areas with nighttime light data and multi-seasonal Landsat imagery across Taiwan from 1998 to 2017
Source: arXiv:2009.07954 source file (2020-09-16)
Supplement: Supplementary file 1 [file Appendix_revised.pdf]

# Detecting and monitoring long-term landslides in urbanized areas with nighttime light data and multi-seasonal Landsat imagery across Taiwan from 1998 to 2017

Tzu-Hsin Karen Chen, Alexander V. Prishchepov, Rasmus Fensholt, Clive E. Sabel

## Supplementary data

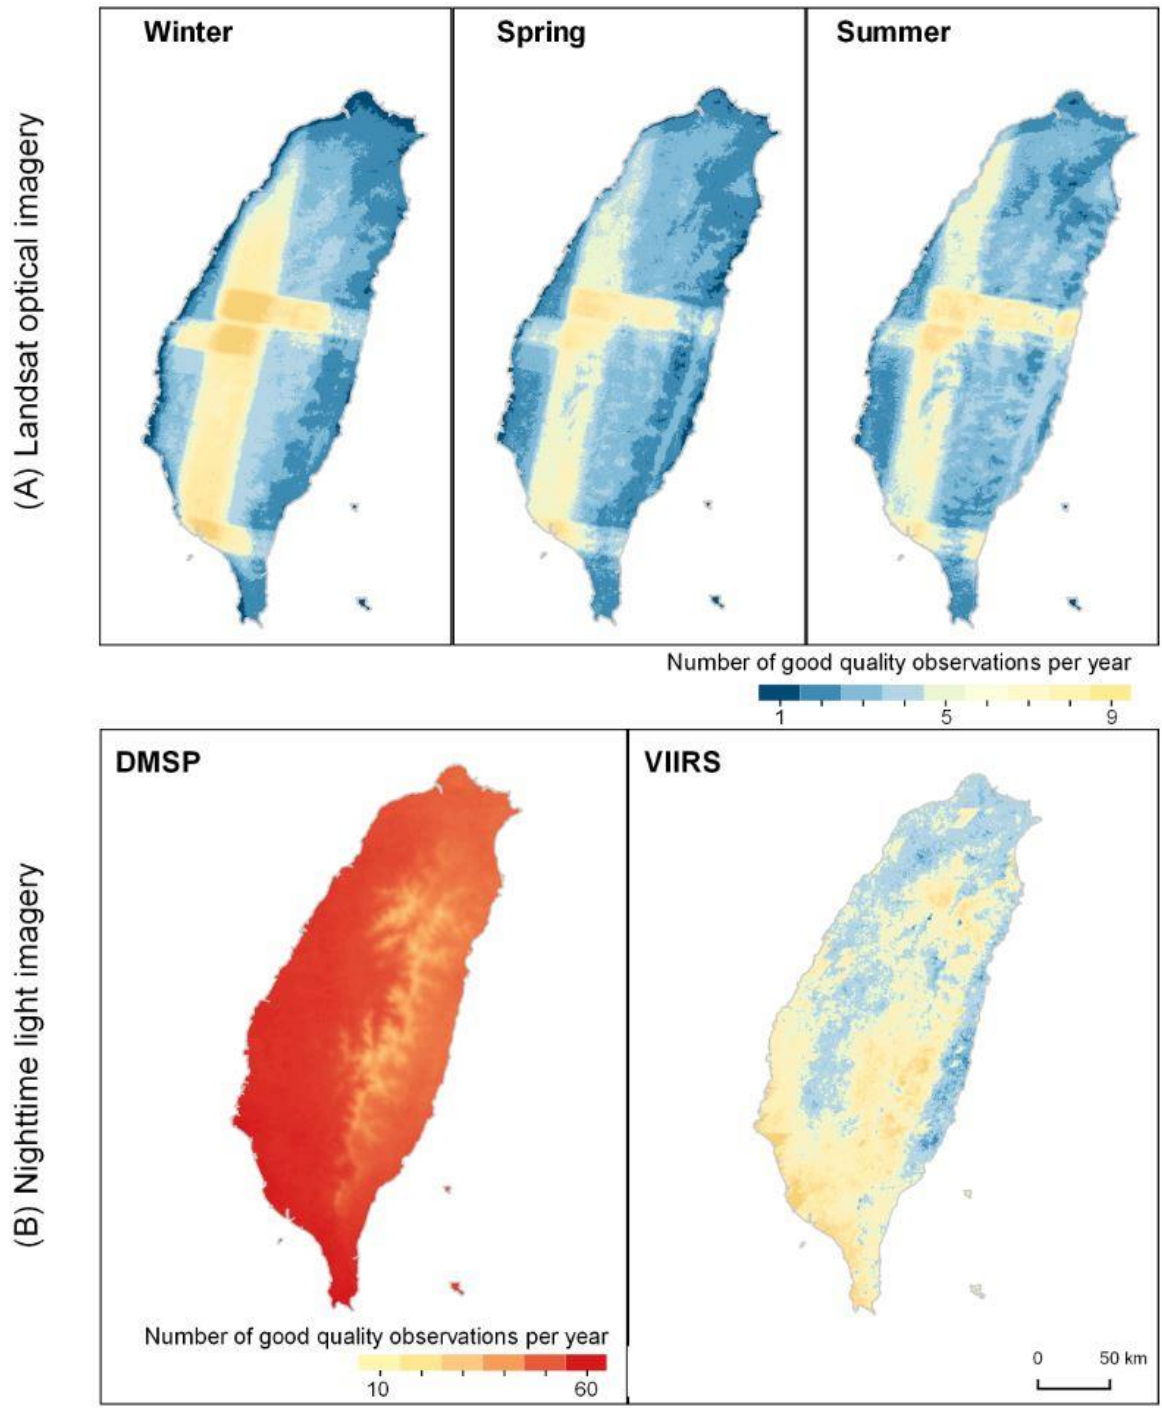

Fig. S1. The observation density of annual variables, (A) Landsat optical imagery (years 1998-2017) and (B) nighttime light imagery (DMSP for 1998-2013 and VIIRS for 2014-2017). The Landsat image availability was assessed for winter, spring, and summer. The DMSP data were annual composites and VIIRS were March composites (avoiding summer).

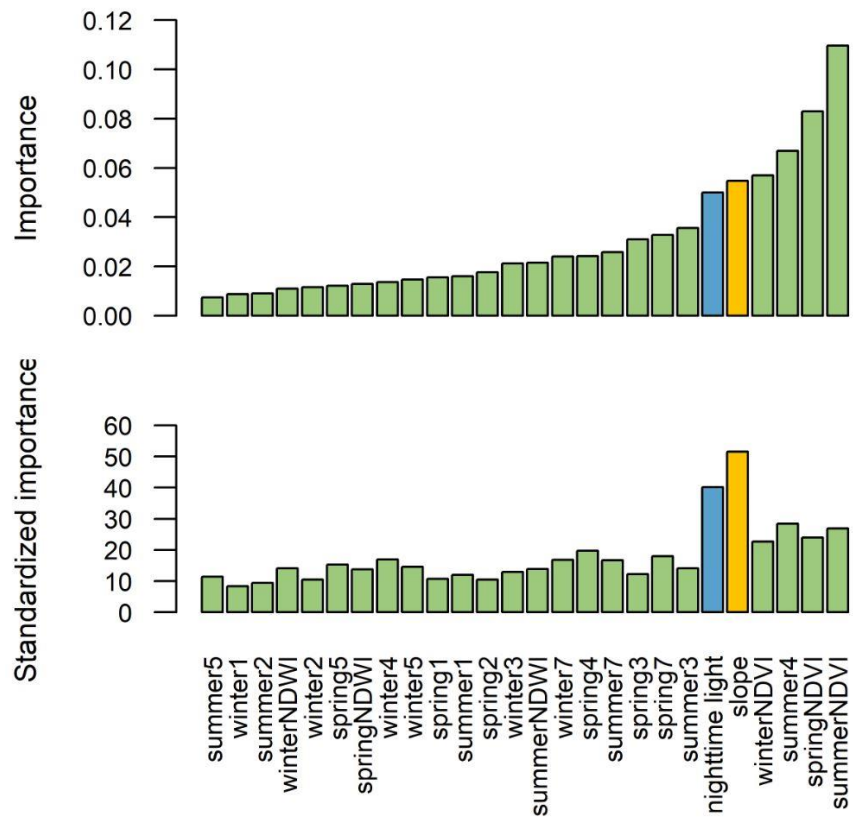

Fig. S2. The importance of a variable was measured as the mean decrease in the producer's accuracy of the landslide class, when the variable in question is excluded. Standardized (Std.) importance is adjusted by standard errors. Variables from ancillary data, nighttime light (blue) and slope (yellow), are highlighted.

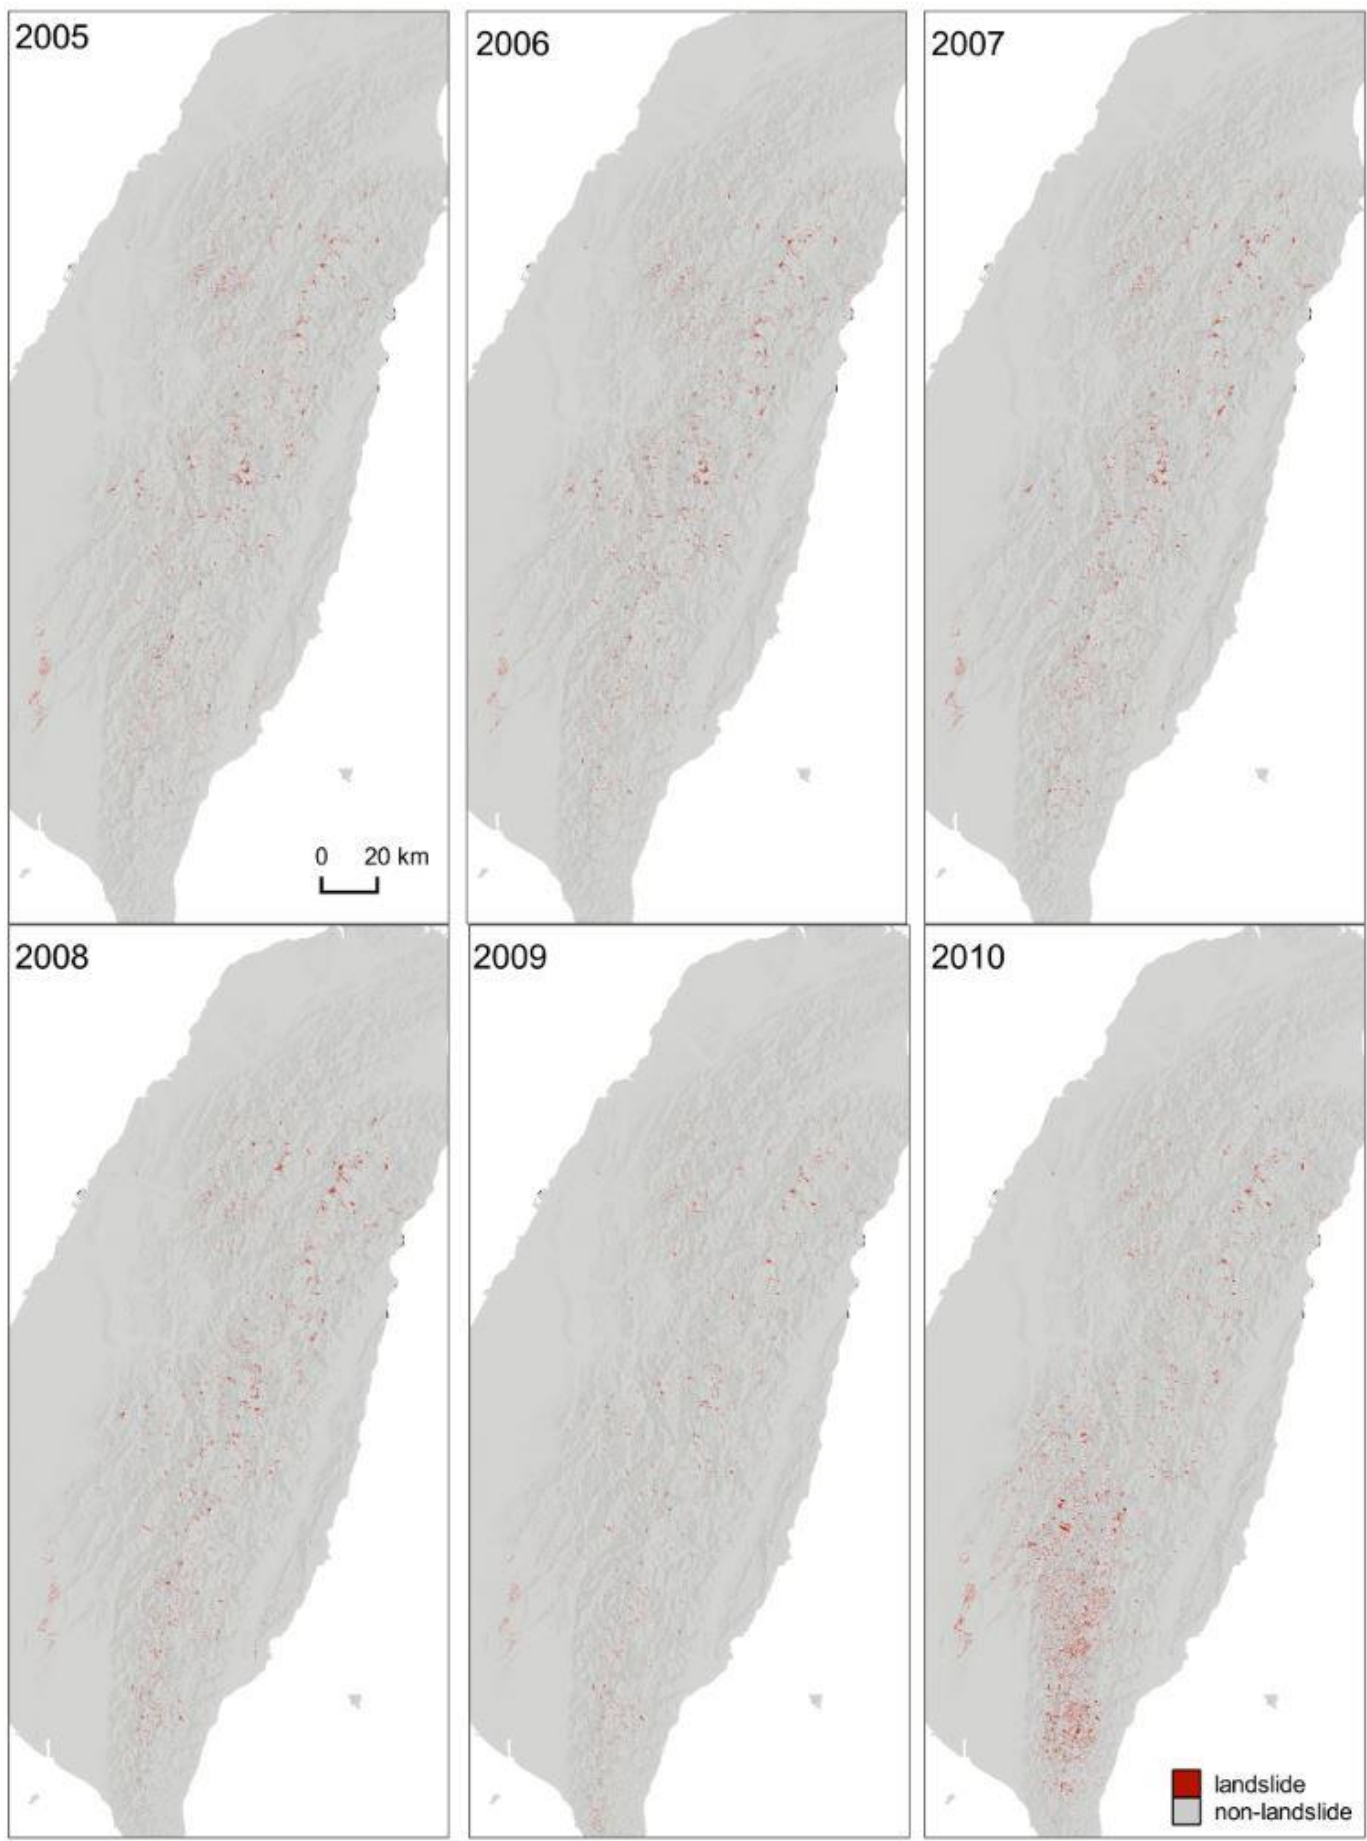

Fig. S3a. Annual reference maps 2005-2010 from the Taiwan Council of Agriculture.

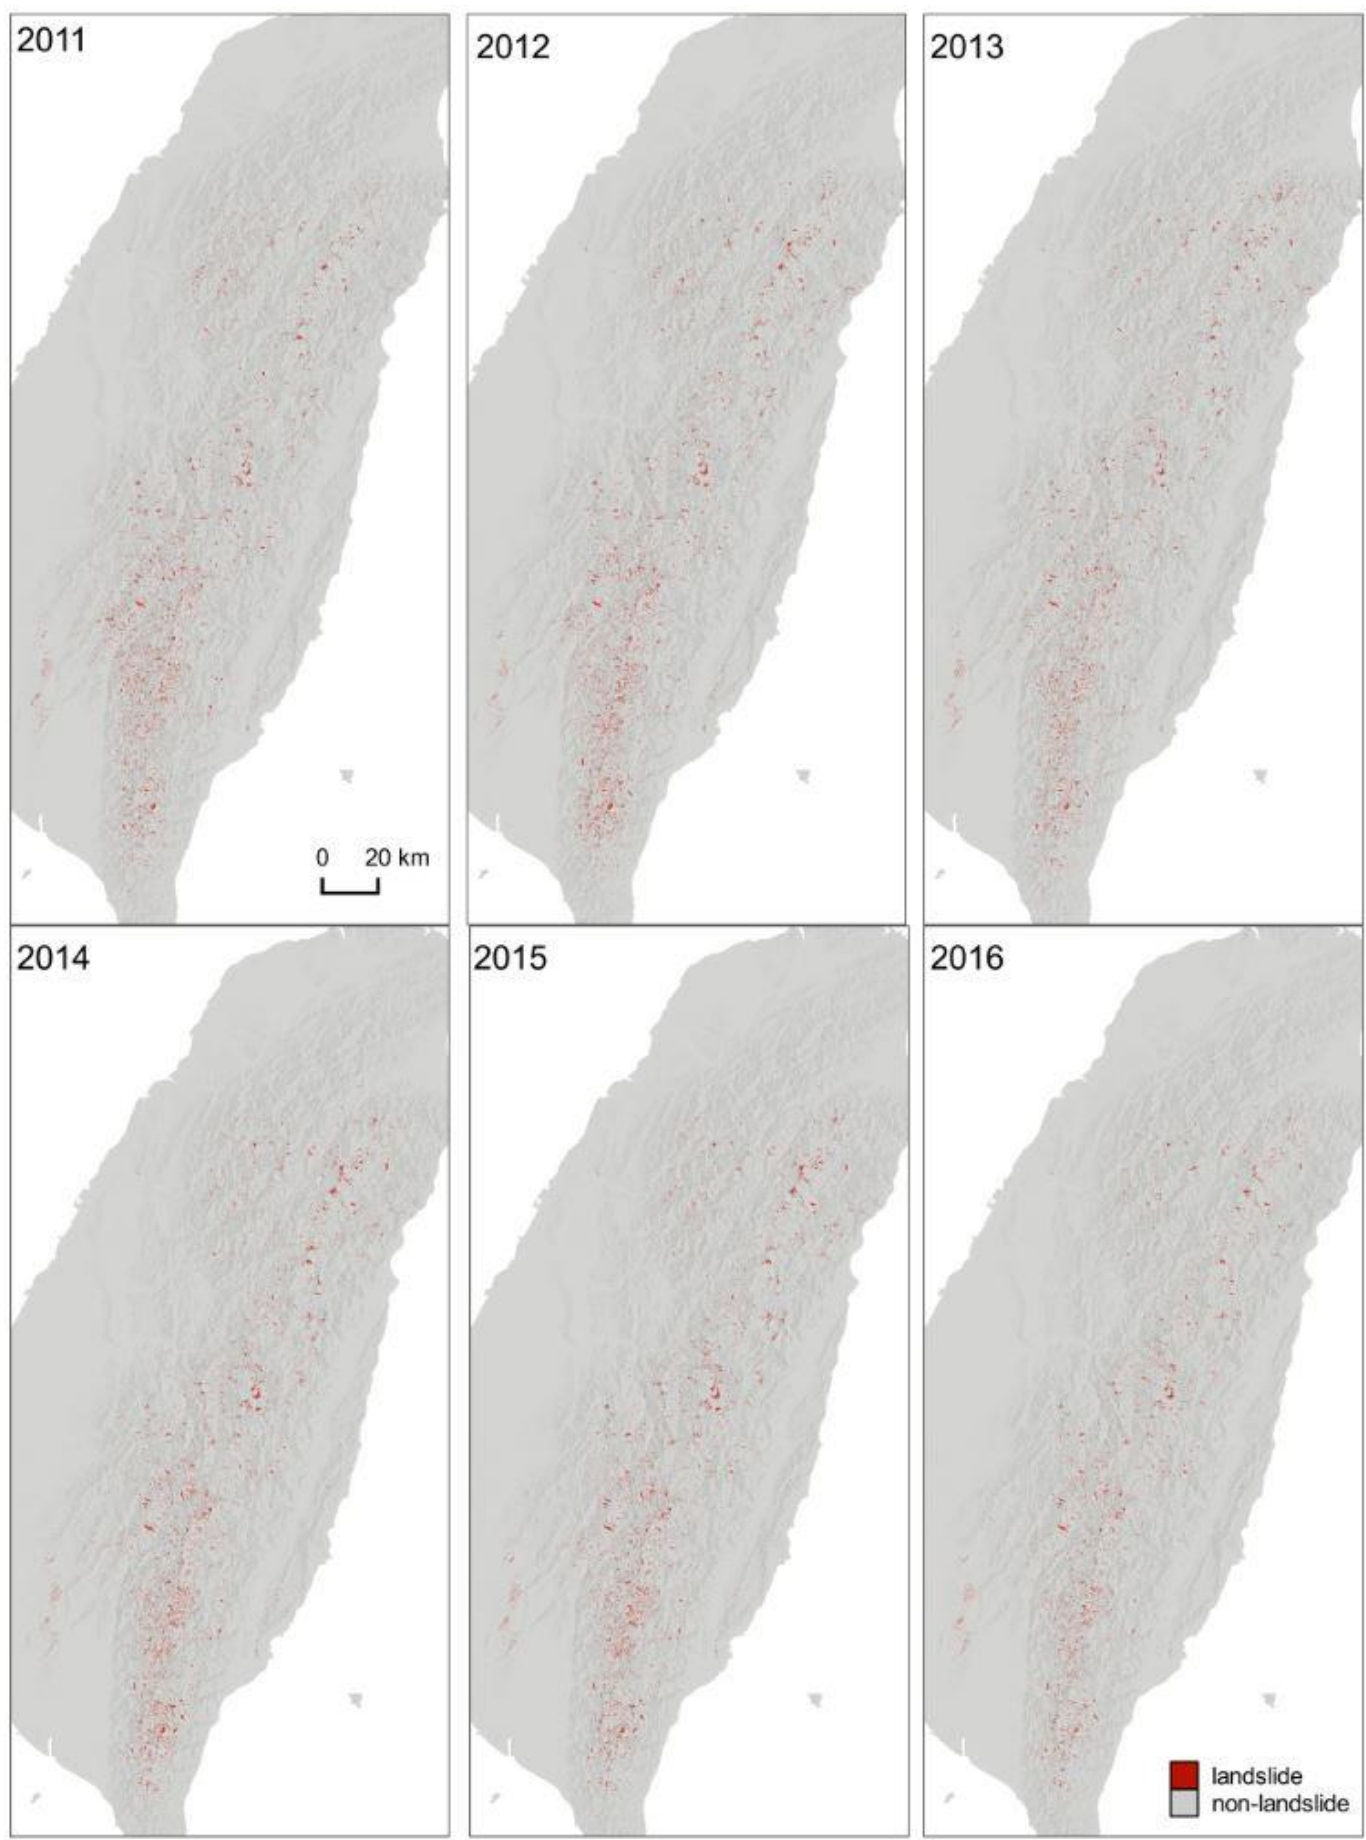

Fig. S3b. Annual reference maps 2011-2016 from the Taiwan Council of Agriculture.
